# Supplementary material for: An Empirical Study on Logging Evolution On Stack Overflow: Trends, Topics, and Challenges
Source: arXiv:2606.00118 source file (2026-05-27)
Supplement: Supplementary file 1 [file 9_Appendix.tex]

% \begin{appendices}
% \section{Figure}
% \label{appendix}
% \begin{figure}[h!]
% \begin{subfigure}[b]{0.8\textwidth}
% \includegraphics[width=\textwidth]{Authors.pdf}
% \caption{Cumulative frequency curve base on \#Authors}
% \label{img1}
% \end{subfigure}
% \hfill
% \begin{subfigure}[b]{0.8\textwidth}
% \includegraphics[width=\textwidth]{Stars.pdf}
% \caption{Cumulative frequency curve base on \#Stars}
% \label{img2}
% \end{subfigure}
% \caption{Cumulative frequency curve of \#Stars and \#Authors}
% \label{img12}
% \end{figure}
% \end{appendices}
